# Supplementary material for: Leveraging Large Language Models to Develop Heuristics for Emerging Optimization Problems
Source: arXiv:2503.03350 source file (2025-03-05)
Supplement: Supplementary file 1 [file appendix.tex]

\section{Appendix}
\label{appendix}

\begin{figure}[hpt]
\centering
\begin{framed}
\begin{justify}
\begin{minipage}{1\textwidth}
\tiny 
\textcolor{brown}{
Act as a professional algorithm designer. 
Design a heuristic for a warehouse optimization problem to minimize the number of reshuffling moves needed to reach a blockage-free state. If a unit load of a lower priority class hinders access to a unit load of a higher priority class, it is deemed blocking. The heuristic should score each warehouse state. Only the warehouse state with the highest score is selected in a tree search procedure.
}
\par
\textcolor{red}{\texttt{'warehouse\_states'}} \textcolor{red}{is represented by a three-level deep nested list. }
\textcolor{red}{The second-level list represents a warehouse state as a list of lists.} 
\textcolor{red}{The third-level list represents a lane of unit loads as a list of integers.} 
\textcolor{red}{The first list index is the outermost slot in the lane, while the highest list index is the innermost slot.} 
\textcolor{red}{Lanes are accessed from the leftmost (outermost) index to the rightmost (innermost).} 
\textcolor{red}{Each integer represents a unit load and its priority class.} 
\textcolor{red}{Unit loads of the same priority class are equal.} 
\textcolor{red}{A \texttt{1} represents the highest priority class.} 
\textcolor{red}{A \texttt{5} represents the lowest priority class.} 
\textcolor{red}{A \texttt{3} represents a priority class lower than \texttt{1} but higher than \texttt{5}.} 
\textcolor{red}{A \texttt{4} represents a priority class lower than \texttt{3} but higher than \texttt{5}.} 
\textcolor{red}{A \texttt{0} represents an empty slot.} 

\textcolor{red}{Each lane must have all \texttt{0}s (empty slots) grouped at the start or have no \texttt{0}s at all, ensuring that if any non-zero elements appear in a lane, all subsequent slots must also be non-zero.} 
\textcolor{red}{Therefore, impossible configurations are:}
\[
\textcolor{red}{[1, 1, 0, 0] \text{ or } [2, 0, 2]}
\]
\textcolor{red}{while possible configurations are:}
\[
\textcolor{red}{[0, 0, 1, 2] \text{ or } [1, 2, 3, 3]}
\]

\textcolor{red}{Examples for blocking unit loads:} \\
\textcolor{red}{In the lane \([0, 4, 1]\), the \texttt{4} blocks access to \texttt{1}.} \\
\textcolor{red}{In the lane \([3, 3, 2]\), the two \texttt{3}s block access to the \texttt{2}.} \\
\textcolor{red}{In the lane \([0, 5, 1, 5, 2]\), the two \texttt{5}s block access to the \texttt{2} and \texttt{1}.} \\
\textcolor{red}{In the lane \([0, 4, 4, 3]\), the two \texttt{4}s block access to the \texttt{3}.} 

\textcolor{red}{First example for \texttt{'warehouse\_states'}}:
\[
\textcolor{red}{
\begin{bmatrix}
[0, 2, 3] & [0, 5, 5] & [5, 1, 1] \\
[0, 2, 3] & [5, 5, 5] & [0, 1, 1] \\
[5, 2, 3] & [1, 5, 5] & [0, 0, 1]
\end{bmatrix}
}
\]

\textcolor{red}{Second example for \texttt{'warehouse\_states'}}:
\[
\textcolor{red}{
\begin{bmatrix}
[2, 2, 3, 5] & [0, 3, 5, 4] & [0, 0, 2, 2] \\
[0, 0, 3, 5] & [2, 3, 5, 4] & [0, 2, 2, 2] \\
[0, 2, 3, 5] & [0, 0, 5, 4] & [3, 2, 2, 2] \\
[0, 0, 3, 5] & [0, 3, 5, 4] & [2, 2, 2, 2]
\end{bmatrix}
}
\]

\textcolor{red}{First example for \texttt{'scores'}}:
\[
\textcolor{red}{[-3, -1, -4]}
\]

\textcolor{red}{Second example for \texttt{'scores'}}:
\[
\textcolor{red}{[0, 1, 3, 1]}
\]

\textcolor{red}{
First, understand the provided problem description and input and output examples. 
Then extract the main constraints of the problem. 
Second, think about how these constraints affect the requested heuristic. }
\textcolor{blue}{Third, describe your new algorithm and main steps in one sentence. The description must be inside a brace. 
Next, implement it in Python as a function named \texttt{select\_next\_move}. 
This function should accept 1 input(s): \texttt{'warehouse\_states'}. 
The function should return 1 output(s): \texttt{'scores'}. 
\texttt{'warehouse\_states'} is the size of all potential warehouse states after all potential reshuffling moves. 
The output named \texttt{'scores'} is the scores for the warehouse states. 
}

\textcolor{violet}{
Note that \texttt{'warehouse\_states'} is a three-level nested list with integers in the third-level sublist. \texttt{'scores'} must be a list of integers or floats. Avoid utilizing any random component, and it is crucial to maintain self-consistency.
Do not give additional explanations.
}
\end{minipage}
\end{justify}
\end{framed}
\caption{Initialization Prompt for the UPMP.}
\label{fig: Initialization_prompt_upmp}
\end{figure}
